# Supplementary material for: End-to-End Multi-View Fusion for 3D Object Detection in LiDAR Point Clouds
Source: arXiv:1910.06528 source file (2019-10-23)
Supplement: Supplementary file 1 [file supplementary.tex]

\section{Supplementary}
\label{sec:supplementary}

\subsection{Hard voxelization design and experiment}
\label{sec:sup_desigh}
One of the inherent design choices for hard voxelization is how to distribute the memory/compute capacity between the maximum number of voxels $K$ sampled from the scene and the maximum number of points $T$ sampled for each voxel. Sampling too few voxels increases the risk that objects of interest will not be covered by enough (or any) voxels. This is especially relevant for smaller objects that don't cover many voxels to begin with and objects farther away where occlusions increase and the point cloud becomes more sparse. On the other hand, sampling too few points from each voxel means that there may not be enough information to sufficiently describe the local spatial details.

To provide a more complete picture of the different voxelization techniques, we also investigated how the hard-voxelization tradeoff between more voxels vs. more points per voxel impacts detection performance. We start with a hard voxelization setting of $K$ = 24k voxels and $T$ = 100 points sampled per voxel. This is similar to the settings used in PointPillars \cite{REF:pointpillars_cvpr2018}, except we increase the number of voxels from the proposed 12k to 24k to account for the larger panoramic detection region in our dataset. From this setup, we progressively increase the number of voxels to 36k and 48k, while decreasing the points-per-voxel by a corresponding amount to keep the total point capacity the same. Finally, we also evaluate a voxelization setting with $K$ = 48k and $T$ = 100, to measure the effect of increasing $T$ at the cost of a higher point buffer capacity.

\label{sec:sup_results}
\textbf{Results}: We evaluate these hard voxelization models on the same large-scale autonomous driving dataset and AP metrics as in Section \ref{sec:od} of the paper.

\begin{table}[h!]
\begin{center}
\begin{tabular}{|l|c|c|c|c|c|c|c|c|}
\hline
\multirow{2}{*}{Method} & \multicolumn{4}{c|}{Vehicle BEV AP (IoU=0.7)}              & \multicolumn{4}{c|}{Vehicle 3D AP (IoU=0.7)}               \\ \cline{2-9}
                      & Overall & 0 - 30  & 30 - 50 & 50 - Inf & Overall & 0 - 30 & 30 - 50 & 50 - Inf \\ \hline
$K$ = 24k, $T$ = 100  & 66.18  & 83.9  & 63.91  & 43.67  & 42.16  & 67.99  & 36.33  & 16.34              \\ \hline
$K$ = 36k, $T$ = 66   & 66.27  & 86.93  & 63.77  & 44.68  & 42.37  & 69.3  & 35.94  & 15.94      \\ \hline
$K$ = 48k, $T$ = 50   & \textbf{69.27}  & \textbf{87.71}  & \textbf{65.09}  & \textbf{46.9}  & \textbf{46.33}  & \textbf{73.08}  & \textbf{42.28}  & \textbf{19.06}      \\ \hline
$K$ = 48k, $T$ = 100  & 68.72  & 87.35  & 64.63  & 46.01  & 43.43  & 68.07  & 36.77  & 17.31      \\ \hline
\end{tabular}
\\
\end{center}
\caption{Comparison of different hard voxelization settings for vehicle detection.}
\label{eval-vehicle}
\end{table}

\begin{table}[h!]
\begin{center}
\begin{tabular}{|l|c|c|c|c|c|c|c|c|}
\hline
\multirow{2}{*}{Method} & \multicolumn{4}{c|}{Pedestrian BEV AP (IoU=0.5)}              & \multicolumn{4}{c|}{Pedestrian 3D AP (IoU=0.5)}               \\ \cline{2-9}
                      & Overall & 0 - 30  & 30 - 50 & 50 - Inf & Overall & 0 - 30 & 30 - 50 & 50 - Inf \\ \hline
$K$ = 24k, $T$ = 100  & 32.02  & 46.67  & 27.56  & 7.332  & 26.75  & 40.93  & 21.28  & 5.739      \\ \hline
$K$ = 36k, $T$ = 66   & 37.62  & 49.14  & 36.79  & \textbf{11.23}  & 27.9  & 42.39  & 23.33  & 4.069      \\ \hline
$K$ = 48k, $T$ = 50   & 38.79  & 50.94  & 35.83  & 10.97  & 29.41  & \textbf{44.0}  & 24.75  & \textbf{6.208}      \\ \hline
$K$ = 48k, $T$ = 100  & \textbf{39.64}  & \textbf{53.65}  & \textbf{40.51}  & 10.65  & \textbf{30.86}  & 43.71  & \textbf{26.73}  & 5.148 \\ \hline
\end{tabular}
\\
\end{center}
\caption{Comparison of different hard voxelization settings for pedestrian detection.}
\label{eval-vehicle}
\end{table}

From the results, we observe that increasing the number of voxels $K$ generally helps performance, even when it comes at the cost of reduced points-per-voxel $T$. This suggests that increasing the voxel-level coverage of the objects in the scene is important for achieving the highest detection performance. A less intuitive observation is that increasing the number of points-per-voxels while keeping the number of voxels fixed does not always yield improvements. In our experiments, the [$K$ = 48k, $T$ = 50] voxelization performs better on vehicle detection than [$K$ = 48k, $T$ = 100], despite the fact that the latter has a larger buffer capacity. This may be due in part to the regularizing effect of stochastically dropping out points, which may serve as a form of data augmentation. This point-level dropout behavior also varies spatially across the scene, happening more in voxels close to the autonomous vehicle (where the point cloud is very dense) and less at longer ranges (where the point cloud becomes sparse relative to the points-per-voxel capacity).
